# Supplementary material for: Robust Learning by Self-Transition for Handling Noisy Labels
Source: arXiv:2012.04337 source file (2021-06-07)

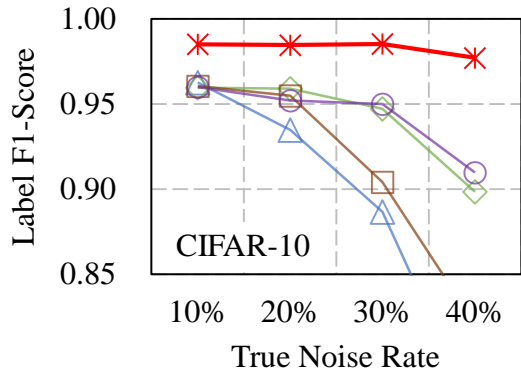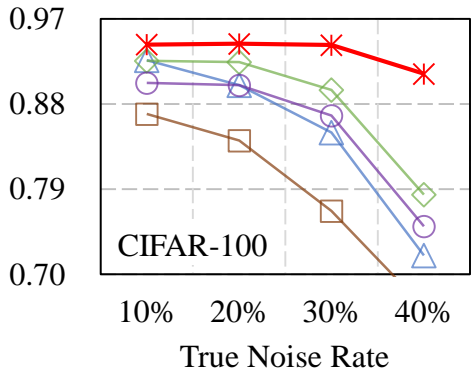

Label F1-Score

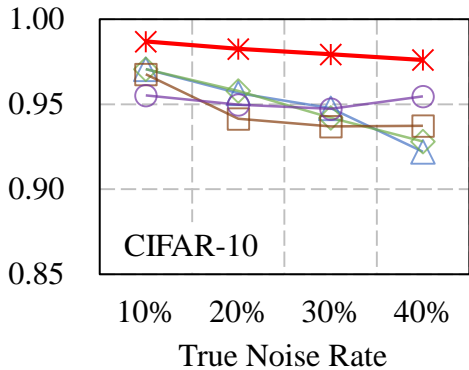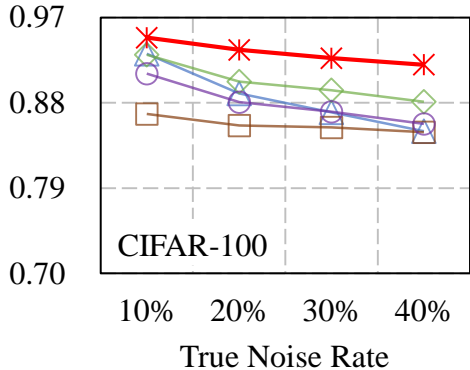

Supplement: Supplementary file 1 [file f_score_v2.pdf]
