# Supplementary material for: Robust Learning by Self-Transition for Handling Noisy Labels
Source: arXiv:2012.04337 source file (2021-06-07)

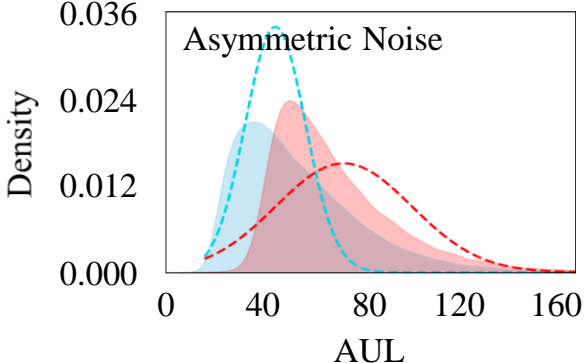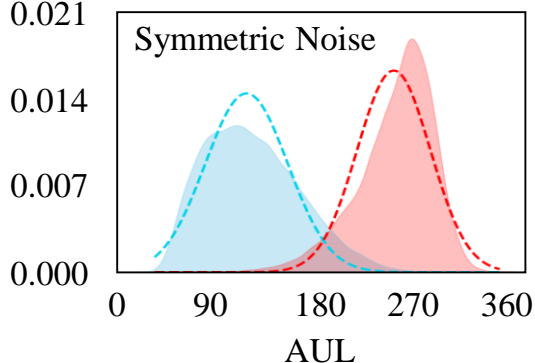

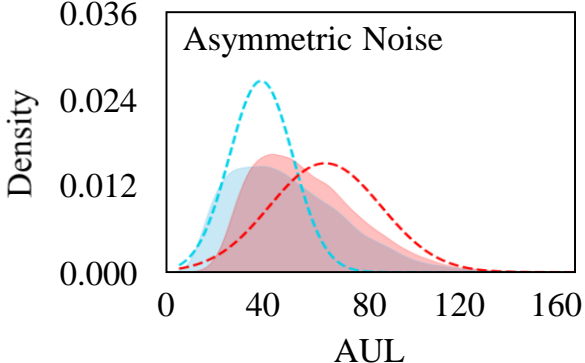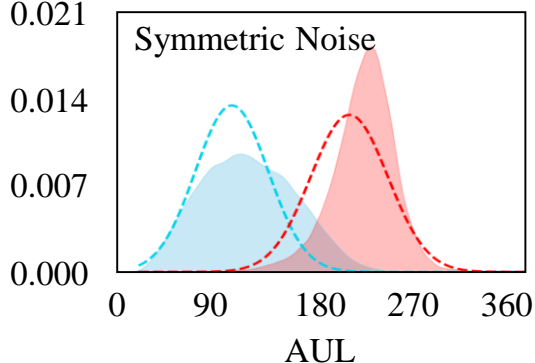

Supplement: Supplementary file 2 [file gmm_analysis.pdf]
